# Supplementary material for: ReTrace: Rejected-Trajectory Conditioning for Speculative Decoding
Source: arXiv:2608.29748 source file (2026-09-05)
Supplement: Supplementary file 1 [file appendix.tex]

\section{Hello World}
%\subsection{Hello World}
